# Supplementary material for: Shielding Atari Games with Bounded Prescience
Source: arXiv:2101.08153 source file (2021-01-22)
Supplement: Supplementary file 1 [file appendix.tex]

\appendix
\section*{Appendix}
%%%%%%
%%%%%%
%%%%%%
\section{General Background on RL}
Often an explicit model of the MDP and its underlying dynamics are unknown. In such cases, RL can be the solution of the choice, where a policy is easily synthesised from an alternating process of interacting with the environment, and learning from the experiences and traces gathered \cite{sutton2018reinforcement}. RL is proved to be able to find optimal policies even for MDPs with entirely unknown behaviour, including an unknown reward function. The promise of RL as a computationally efficient method to solve unknown MDPs originates from its ability to guide the experience gathering process, often referred to as `exploration', towards promising parts of the state-space. Interestingly, RL employs the very same policy that is being learned to guide the exploration. This if often referred to as `exploitation' of the knowledge of the agent, and can quickly lead to competent policies. However,  in order to efficiently find a good policy care must be taken to balance exploration and exploitation. It is well-known that if the state space is not sufficiently explored there is always a risk of not finding the optimal solutions at all, and getting stuck in local optimum.

A classic example of a model-free RL is Q-learning (QL) \cite{watkins1992q}, which uses a similar update rule as that in value iteration. QL assumes no access to the transition probabilities of the MDP and instead only updates along the exploration traces. More formally, QL keeps an action-value function $Q:S\times A\to \mathbb{R}$ which assigns an estimated value to performing a particular action at a particular state. The $Q$-function is iteratively updated from experience in the environment after moving from $s$ to $s'$ by taking action $a$ and obtaining reward $r$:
\begin{equation}\label{Q'}
Q'(s,a) = r + \gamma \max_{a'\in A}Q(s',a'),
\end{equation} 
as the new estimate of how rewarding it is to take action $a$ at state $s$. The algorithm then updates the $Q$-function by taking a weighted average of this updated value and the old one
$$Q(s,a) = (1-\alpha)Q(s,a)+ \alpha Q'(s,a),$$ 
where $\alpha$ is referred to as the learning rate, and determines how much to weigh the new estimate against the old. As long as continual exploration is ensured and the learning rate is tuned appropriately, QL provably converges to an optimal $Q$-function under mild assumptions \cite{watkins1992q}.

%%%%%%
%%%%%%
%%%%%%
\section{Training Conventions and Preprocessing in Atari}
Theoretical analysis and training on Atari will often consider it as a large MDP with full frame and action histories as states \cite{NatureDQN} instead of a POMDP, since most RL theory is based on full observability. The determinism of the Atari games justifies this conversion, since a sequence of actions $a_1,a_2,...,a_n$ uniquely determines the resulting state $s_n$. When training Deep RL systems the full history is not used as the observation since it would become much too large and most Deep RL methods want a fixed-size observation. Sometimes recurrent networks are used, but the most common method is to simply drop all but the $n$ most recent frame observations, which are stacked into a fixed-length observation and passed to the agent (commonly $n=4$). This practice along with a series of additional preprocessing steps were first established in the seminal DQN paper \cite{NatureDQN}, and the majority of algorithms use a similar (but not necessarily identical) approach since then. These steps and their motivation will now be described.
\subsection{Frameskips}
The first preprocessing step is that frameskips (often 4) are often introduced, where the agent only acts on every 4th frame and their latest action repeated in between, so that the sequence of observations $o$ are given by the sequence of frames $f$ as $$o_0=f_0,o_1=f_4,o_2=f_8,...o_i=f_{4i}$$The primary justification is that the games rarely need faster or more precise responses (since they are built for humans), and that this allows for training on four times the number of episodes in almost the same amount of time. Additionally some games can benefit from the way frame-skips compress temporal distance\cite{braylan2015frame}, sometimes even benefiting from very high frame-skips of 60 frames (though this obviously degrades performance heavily in reflex-based games that require quick and precise movement).

\subsection{Framestacking}
After applying the frameskips, it has become standard to also stack the last 4 observations together in parallel. Since this stacks previous observations and not frames it combines with frame-skips to create observations
$$o_i = (f_{4i},f_{4i-4},f_{4i-8},f_{4i-12}).$$Since many algorithms are memoryless this can help significantly with exposing temporal information, and is the main way the partially observable nature of the games is addressed. 

\subsection{Max-Pooling}
A problem when observing only isolated frames in Atari, especially when using frame-skips, is that many games utilise graphical flickering, where images are only displayed on e.g. every other frame, to be able to draw more objects and save performance (or for graphical effect). This was perhaps done because such rapid flickering is difficult for human perception to notice and because the games were intended to be displayed on CRT televisions whose phosphor-based screens often had long afterglow~\cite{machado2017revisiting}. When extracting individual frames this means that sometimes important entities in the game will not show up at all. Without frameskip sufficient framestacking would be enough to resolve this, but when frameskips are used the periods of the flickering and frameskips risk aligning such that the entities never show up in the observation. 

In order to resolve this a max-pooling or color-averaging operation will often be applied combining 2 or more subsequent frames by taking the element-wise maximum/average. A max-pool of 2 in combination with frame-skips and frame-stacking of 4 results in observations 
\begin{align}
\begin{aligned}
o_i=&\Big(\max(f_{4i},f_{4i-1}),\max(f_{4i-4},f_{4i-5}),\\
&\max(f_{4i-8},f_{4i-9}),\max(f_{4i-12},f_{4i-13})\Big).
\end{aligned}
\end{align}
$$$$
\subsection{Greyscale and downscale}
Instead of working with full 210x160 128-color images it is common to downscale them to greyscale 84x84 images. It seems the information lost from this transformation is compensated for by the reduced amount of redundant information. Different code-bases and algorithms will often use slightly different downsampling operations, and since algorithms overfit to the specifics of the downsampling this can cause large performance drops, which can be an obstacle to reproduction.

\subsection{Episode ends}

There is some variation in how episode ends are determined---while a game over screen is always agreed to mean the end of an episode, various authors also introduce additional episode-end conditions. Most common is artificially ending a game after a certain number of frames: 5 minutes (18,000 frames at 60Hz) or 30 minutes (108,000 frames) are common choices. One reason to do this is that if a game goes on for a long time it is likely because the agent has gotten stuck or become inactive, and continuing to learn from that game could negatively impact training. However this has obvious negative impacts as well, putting a cap on maximum performance in many games and incentivising short-sighted behaviour. It also makes it more difficult to compare results when evaluation uses different maximum game lengths \cite{AtariTrainProtocol}.

It is also somewhat common to end the training episode whenever the agent dies, even if they still have lives left. This can help the agent learn to avoid death, since the feedback from dying is immediate instead of delayed, and it aligns with the way some games treat a death as a 'soft-reset', putting many entities back in their starting positions. However in recent years a consensus has started building that terminating episodes on death is arbitrary, can hurt training in the long run and makes comparison more difficult and should generally be avoided \cite{machado2017revisiting} \cite{AtariTrainProtocol}. 

\subsection{Reward normalisation}
It is generally considered part of the challenge to use the same hyperparameters for all games when training on Atari, to avoid artificial inflation of results by overfitting to particular games. This can cause problems though, since games generally have wildly different average magnitudes of rewards, so various forms of normalisation are commonly applied. The simplest and perhaps most common is reward-clipping, where all rewards are normalised to $\{-1,+1\}$ depending on their sign. While this has been effective empirically it has been criticised for changing optimal behaviour in many games~\cite{AtariTrainProtocol}.

%%%%%%
%%%%%%
%%%%%%
\section{Safety Properties} \label{sec:appendix-c}
The following criteria were taken into account when specifying the safety properties: 
\begin{enumerate}
	\item The property should be possible to satisfy.
	\item The property should not be trivially satisfied, e.g., it should not be satisfied by a random agent. Otherwise, checking such property is useless.
	\item The property should be plausibly satisfied by an optimal policy with respect to the reward, meaning entering an unsafe state should never be beneficial.
	\item The property needs to be relatively simple to construct a labelling function for. 
	\item The property should be simple and 'natural' whenever possible.
\end{enumerate}
The first two desiderata are fairly obvious, and it is generally possible to determine if a property satisfies them with some experience of the game in question. 

The third desiderata is a bit vague, but important given that we investigate agents trained purely to optimise reward. If the property is directly at odds with maximising reward then satisfying it is not part of 'intended generalisation'. Thus, we instead would like to deal with properties that are intuitively part of maximising the reward.

Finally the fifth desiderata is perhaps the most nebulous, and mostly serves as a guiding principle to justify which properties are chosen among the many possible which satisfy the other four desiderata. For instance, a property like 'do not run into an obstacle after having run back and forth seven times' might satisfy the previous four desiderata, and yet we prefer the simpler 'do not run into an obstacle'. As a small attempt to assess whether there was any agreement about what 'naturalness' and 'simplicity' meant for Atari properties we asked 4 others to independently construct properties for 5 games, and 6 out of the 9 properties suggested independently were identical. A contribution to this large consensus is that many games have a very natural property of avoiding death/losing a life.

Based on these criteria a list of 84 properties are outlined and put in the spreadsheet, and prioritised based on ease of implementation and how well they fulfill the desiderata.

\subsection{Properties Considerations}
While we tried to structure the creation of properties as much as possible, they are ultimately picked in an ad-hoc manner. The labelling functions are also coded by hand in occasionally complex ways and might contain errors. Our approach to this is to take care in our analysis to look at concrete traces and evaluate qualitatively whether satisfying/not satisfying a particular property actually reflects the sort of safe/unsafe behaviour that we are interested in, or whether it reflects a misspecification or poorly defined property.  
\subsubsection{Difficult Properties}
Many of the properties, such as avoiding death in many games, are extremely demanding to always avoid, even for a human player. However, the limit maximum frames of our environment make these more feasible to satisfy.
\subsubsection{Misspecification}
Misspecification in the labelling function are critical. In order to minimise this risk we set up our framework for easy testing of properties both using human play, random play or play by trained policies, and made sure to evaluate whether the label was being applied to the correct states.

\subsection{Unsafe States During No-ops}
The model checker, as described above, assumes the game starts with the state $s_i$ reached after completing the initial $i$ no-ops, and would ignore any unsafe states arrived at during these no-ops. As expected from what is at most a half-second delay however, this turns out to not occur for any number of no-ops on any of our properties.
